# Supplementary material for: Transport and dispersion of active particles in periodic porous media
Source: arXiv:1809.00086 ancillary file (2019-01-09)
Supplement: Supplementary file 1 [file SupplementalInformation.pdf]

# Supplemental Information

## Asymptotic transport and dispersion of active particles in periodic porous media

Roberto Alonso-Matilla, Brato Chakrabarti, and David Saintillan

*Department of Mechanical and Aerospace Engineering,  
University of California San Diego, 9500 Gilman Drive, La Jolla, CA 92093, USA*

### I. Macro-continuum model

We provide details of the macro-continuum model used to estimate the mean velocity  $\bar{\mathbf{U}}$  and dispersivity dyadic  $\bar{\mathbf{D}}$ . The method extends Brenner's generalized Taylor dispersion theory [1] to the case of polar active particles with a unit director  $\mathbf{p}$ .

#### A. Local moments of the conditional probability

For a fixed cell  $(\alpha, \beta)$  (see Fig. 1 below for nomenclature), the conditional probability density  $\psi$  satisfies the following Fokker-Planck equation:

$$\frac{\partial \psi}{\partial t} + \nabla_r \cdot \mathbf{J} + \nabla_p \cdot \mathbf{j} = \delta_{\alpha 0} \delta_{\beta 0} \delta(\mathbf{r} - \mathbf{r}_0) \delta(\mathbf{p} - \mathbf{p}_0) \delta(t). \quad (1)$$

It is normalized in such a way that the sum of the probabilities over all possible configurations is one after the swimmer is set free:

$$\sum_{\alpha, \beta=-\infty}^{\infty} \int_{S_{\alpha\beta}} \int_{\Omega} \psi(\mathbf{R}_{\alpha\beta}, \mathbf{r}, \mathbf{p}, t | \mathbf{r}_0, \mathbf{p}_0) d\mathbf{p} d^2\mathbf{r} = \begin{cases} 1 & \text{for } t \geq 0, \\ 0 & \text{for } t < 0. \end{cases} \quad (2)$$

Convergence of the previous infinite sum requires that

$$\psi(\mathbf{R}_{\alpha\beta}, \mathbf{r}, \mathbf{p}, t | \mathbf{r}_0, \mathbf{p}_0) \rightarrow 0 \quad \text{as } \alpha, \beta \rightarrow \pm\infty. \quad (3)$$

Subsequent convergence of the probability moments defined below will require that for any integer  $n \geq 0$

$$|\mathbf{R}_{\alpha\beta}|^n \psi \rightarrow 0 \quad \text{and} \quad |\mathbf{R}_{\alpha\beta}|^n \mathbf{J} \rightarrow \mathbf{0} \quad \text{as } \alpha, \beta \rightarrow \pm\infty. \quad (4)$$

Boundary conditions for  $\psi$  need to be specified on the obstacle boundaries as well as cell edges. The no-flux condition at the obstacle walls reads

$$\mathbf{n}_w \cdot \mathbf{J} = 0 \quad \text{on } \partial C_w, \quad (5)$$

where  $\mathbf{n}_w$  is the unit vector normal to the wall. Continuity across the cell edges requires

$$\psi(\mathbf{R}_{\alpha\beta}, \mathbf{r}, \mathbf{p}, t) = \psi(\mathbf{R}_{\alpha+1\beta}, \mathbf{r} - L_x \mathbf{e}_x, \mathbf{p}, t) \quad \text{on } \mathbf{r} \in \partial C_{\alpha+\beta}, \quad (6a)$$

$$\psi(\mathbf{R}_{\alpha\beta}, \mathbf{r}, \mathbf{p}, t) = \psi(\mathbf{R}_{\alpha\beta+1}, \mathbf{r} - L_y \mathbf{e}_y, \mathbf{p}, t) \quad \text{on } \mathbf{r} \in \partial C_{\alpha\beta+}, \quad (6b)$$

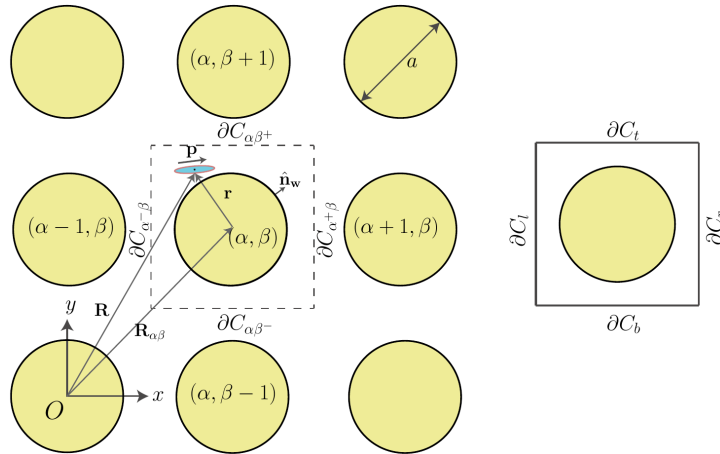

FIG. 1: Geometry of the lattice and associated nomenclature in the case of circular pillars.

where we omit arguments  $\mathbf{r}_0$  and  $\mathbf{p}_0$  for brevity. Likewise, continuity of the particle translational flux crossing the cell edges reads:

$$\nabla_r \psi(\mathbf{R}_{\alpha\beta}, \mathbf{r}, \mathbf{p}, t) = \nabla_r \psi(\mathbf{R}_{\alpha+1\beta}, \mathbf{r} - L_x \mathbf{e}_x, \mathbf{p}, t) \quad \text{on} \quad \mathbf{r} \in \partial C_{\alpha+\beta}, \quad (7a)$$

$$\nabla_r \psi(\mathbf{R}_{\alpha\beta}, \mathbf{r}, \mathbf{p}, t) = \nabla_r \psi(\mathbf{R}_{\alpha\beta+1}, \mathbf{r} - L_y \mathbf{e}_y, \mathbf{p}, t) \quad \text{on} \quad \mathbf{r} \in \partial C_{\alpha\beta+}. \quad (7b)$$

We define the  $k$ th-order polyadic local moment of  $\psi$  as

$$\psi_k(\mathbf{r}, \mathbf{p}, t | \mathbf{r}_0, \mathbf{p}_0) = \sum_{\alpha, \beta = -\infty}^{\infty} \underbrace{\mathbf{R}_{\alpha\beta} \cdots \mathbf{R}_{\alpha\beta}}_{k \text{ times}} \psi(\mathbf{R}_{\alpha\beta}, \mathbf{r}, \mathbf{p}, t | \mathbf{r}_0, \mathbf{p}_0) \quad k = 0, 1, 2, \dots \quad (8)$$

Taking moments of the Fokker-Planck equation (1) provides conservation equations for the  $\psi_k$ 's:

$$\frac{\partial \psi_k}{\partial t} + \nabla_r \cdot \mathbf{J}_k + \nabla_p \cdot \mathbf{j}_k = \delta_{k0} \delta(\mathbf{r} - \mathbf{r}_0) \delta(\mathbf{p} - \mathbf{p}_0) \delta(t), \quad (9)$$

where  $\mathbf{J}_k$  and  $\mathbf{j}_k$  are the local moments of the translational and orientational fluxes, respectively. In dimensionless form, they read

$$\mathbf{J}_k = [\text{Pe}_s \mathbf{p} + \mathbf{u}(\mathbf{r})] \psi_k - \kappa^2 \nabla_r \psi_k, \quad (10a)$$

$$\mathbf{j}_k = \frac{1}{2} [\boldsymbol{\Omega}(\mathbf{r}) \times \mathbf{p}] \psi_k - \nabla_p \psi_k, \quad (10b)$$

where  $\boldsymbol{\Omega}(\mathbf{r}) = \nabla_r \times \mathbf{u}(\mathbf{r})$  is the local fluid vorticity. From the pre-initial condition, we require  $\psi_k = \mathbf{0}$  for  $t < 0$ . Eq. (5) implies a no-flux condition for the local moments at the obstacle walls:  $\mathbf{n}_w \cdot \mathbf{J}_k = 0$  on  $C_w$ .

In order to determine  $\bar{\mathbf{U}}$  and  $\bar{\mathbf{D}}$ , our theoretical model in Sec. IC will require boundary conditions on the first three local moments ( $k = 0, 1, 2$ ). A boundary condition on  $\psi_0$  can first be obtained by calculating the zeroth moment of Eqs. (6a)–(6b). First, with Eq. (6a):

$$\sum_{\alpha, \beta = -\infty}^{\infty} \psi(\mathbf{R}_{\alpha\beta}, \mathbf{r}, \mathbf{p}, t) = \sum_{\alpha, \beta = -\infty}^{\infty} \psi(\mathbf{R}_{\alpha+1\beta}, \mathbf{r} - L_x \mathbf{e}_x, \mathbf{p}, t) \quad \text{on} \quad \mathbf{r} \in \partial C_{\alpha+\beta}.$$

Applying translational invariance of the dummy index  $\alpha$  on the right side and using the definition in Eq. (8) yields

$$\psi_0(\mathbf{r}, \mathbf{p}, t) = \psi_0(\mathbf{r} - L_x \mathbf{e}_x, \mathbf{p}, t) \quad \text{on} \quad \mathbf{r} \in \partial C_{\alpha+\beta}. \quad (11)$$

A similar procedure applied to Eq. (6b) also provides:

$$\psi_0(\mathbf{r}, \mathbf{p}, t) = \psi_0(\mathbf{r} - L_y \mathbf{e}_y, \mathbf{p}, t) \quad \text{on} \quad \mathbf{r} \in \partial C_{\alpha\beta+}. \quad (12)$$

Boundary conditions on  $\psi_1$  and  $\psi_2$  can similarly be obtained by taking the first and second moments of Eqs. (6a)–(6b). After simplifications, the boundary conditions on  $\psi_1$  read

$$\psi_1(\mathbf{r}, \mathbf{p}, t) - \psi_1(\mathbf{r} - L_x \mathbf{e}_x, \mathbf{p}, t) = (\mathbf{r} - L_x \mathbf{e}_x) \psi_0(\mathbf{r} - L_x \mathbf{e}_x, \mathbf{p}, t) - \mathbf{r} \psi_0(\mathbf{r}, \mathbf{p}, t) \quad \text{on} \quad \mathbf{r} \in \partial C_{\alpha+\beta}, \quad (13)$$

$$\psi_1(\mathbf{r}, \mathbf{p}, t) - \psi_1(\mathbf{r} - L_y \mathbf{e}_y, \mathbf{p}, t) = (\mathbf{r} - L_y \mathbf{e}_y) \psi_0(\mathbf{r} - L_y \mathbf{e}_y, \mathbf{p}, t) - \mathbf{r} \psi_0(\mathbf{r}, \mathbf{p}, t) \quad \text{on} \quad \mathbf{r} \in \partial C_{\alpha\beta+}, \quad (14)$$

while those on  $\psi_2$  read

$$\psi_2(\mathbf{r}, \mathbf{p}, t) - \psi_2(\mathbf{r} - L_x \mathbf{e}_x, \mathbf{p}, t) = \frac{\psi_1(\mathbf{r}) \psi_1(\mathbf{r})}{\psi_0(\mathbf{r})} - \frac{\psi_1(\mathbf{r} - L_x \mathbf{e}_x) \psi_1(\mathbf{r} - L_x \mathbf{e}_x)}{\psi_0(\mathbf{r} - L_x \mathbf{e}_x)} \quad \text{on} \quad \mathbf{r} \in \partial C_{\alpha+\beta}, \quad (15)$$

$$\psi_2(\mathbf{r}, \mathbf{p}, t) - \psi_2(\mathbf{r} - L_y \mathbf{e}_y, \mathbf{p}, t) = \frac{\psi_1(\mathbf{r}) \psi_1(\mathbf{r})}{\psi_0(\mathbf{r})} - \frac{\psi_1(\mathbf{r} - L_y \mathbf{e}_y) \psi_1(\mathbf{r} - L_y \mathbf{e}_y)}{\psi_0(\mathbf{r} - L_y \mathbf{e}_y)} \quad \text{on} \quad \mathbf{r} \in \partial C_{\alpha\beta+}. \quad (16)$$

It is convenient to introduce the jump operator  $\llbracket \cdot \rrbracket$  for an arbitrary variable  $\mathbf{f}$ , which we define as

$$\llbracket \mathbf{f} \rrbracket = \begin{cases} \mathbf{f}(\mathbf{r}, \mathbf{p}, t) - \mathbf{f}(\mathbf{r} - L_x \mathbf{e}_x, \mathbf{p}, t) & \text{for } \mathbf{r} \in \partial C_r, \\ \mathbf{f}(\mathbf{r}, \mathbf{p}, t) - \mathbf{f}(\mathbf{r} - L_y \mathbf{e}_y, \mathbf{p}, t) & \text{for } \mathbf{r} \in \partial C_t. \end{cases} \quad (17)$$

With this notation, the boundary conditions in Eqs. (11)–(16) summarize as follows:

$$\llbracket \psi_0 \rrbracket = 0, \quad (18a)$$

$$\llbracket \psi_1 \rrbracket = -\llbracket \mathbf{r} \psi_0 \rrbracket, \quad (18b)$$

$$\llbracket \psi_2 \rrbracket = \llbracket \psi_1 \psi_1 / \psi_0 \rrbracket. \quad (18c)$$

Following a similar procedure, we can obtain the boundary conditions associated to Eqs. (7a) and (7b). The final result is:

$$\llbracket \nabla_r \psi_0 \rrbracket = \mathbf{0}, \quad (19a)$$

$$\llbracket \nabla_r \psi_1 \rrbracket = -\llbracket \nabla_r (\mathbf{r} \psi_0) \rrbracket, \quad (19b)$$

$$\llbracket \nabla_r \psi_2 \rrbracket = \llbracket \nabla_r (\psi_1 \psi_1 / \psi_0) \rrbracket, \quad (19c)$$

which coincide with those obtained by Brenner [1] for passive particulate systems. Upon taking the asymptotic limits of the local moments, it will be useful to rewrite the first-order boundary conditions in the form:

$$\llbracket \psi_1 \rrbracket = -\llbracket \mathbf{r} \rrbracket \psi_0, \quad \llbracket \nabla_r \psi_1 \rrbracket = -\nabla_r \psi_0 \llbracket \mathbf{r} \rrbracket, \quad (20)$$

where we have made use of the zeroth-order conditions.

### B. Global moments of the conditional probability

We define the  $k$ th-order dyadic global moment  $\mathbf{M}_k$  as the spatial and orientational average of the corresponding local moment  $\psi_k$ :

$$\mathbf{M}_k(t|\mathbf{r}_0, \mathbf{p}_0) = \int_{S_t} \int_{\Omega} \psi_k(\mathbf{r}, \mathbf{p}, t|\mathbf{r}_0, \mathbf{p}_0) d\mathbf{p} d^2\mathbf{r} \quad k = 0, 1, 2... \quad (21)$$

The zeroth-order global moment derives immediately from the normalization condition in Eq. (2):

$$M_0 = \begin{cases} 1 & \text{for } t \geq 0, \\ 0 & \text{for } t < 0. \end{cases} \quad (22)$$

A differential equation for  $\mathbf{M}_k(t)$  can be obtained by taking the temporal derivative of Eq. (21) and combining it with Eq. (9):

$$\frac{d\mathbf{M}_k}{dt} = \int_{S_t} \int_{\Omega} [-\nabla_r \cdot \mathbf{J}_k - \nabla_p \cdot \mathbf{j}_k + \delta_{k0} \delta(\mathbf{r} - \mathbf{r}_0) \delta(\mathbf{p} - \mathbf{p}_0) \delta(t)] d\mathbf{p} d^2\mathbf{r}.$$

The integral of the orientational flux divergence vanishes. Applying the divergence theorem then gives:

$$\frac{d\mathbf{M}_k}{dt} = - \int_{\Omega} \oint_{\partial C} \mathbf{J}_k \cdot \mathbf{n} d\ell d\mathbf{p} + \delta_{k0} \delta(t), \quad (23)$$

where  $\mathbf{n}$  is the outward unit normal along the cell edges, and where the closed line integral represents the sum of the integrals over all four edges (see Fig. 1):

$$\oint_{\partial C} = \int_{\partial C_r} + \int_{\partial C_t} + \int_{\partial C_l} + \int_{\partial C_b}$$

By making use of the jump operator defined in Eq. (17) we can rewrite Eq. (23) as

$$\frac{d\mathbf{M}_k}{dt} = - \int_{\Omega} \int_{\partial C_r + \partial C_t} \llbracket \mathbf{J}_k \rrbracket \cdot \mathbf{n} d\ell d\mathbf{p} + \delta_{k0} \delta(t). \quad (24)$$

### C. Asymptotic analysis at long times

We now proceed to obtain expressions for the mean velocity  $\bar{\mathbf{U}}$  and dispersivity tensor  $\bar{\mathbf{D}}$  by analysis of the long-time moments.

(1) *Mean velocity:* To determine the mean transport velocity  $\bar{\mathbf{U}}$  we first calculate the average displacement of a swimmer at time  $t$  as

$$\overline{\Delta \mathbf{R}}(t) = \overline{\mathbf{R}(t) - \mathbf{R}(0)} = \sum_{\alpha, \beta = -\infty}^{\infty} \int_{S_{\alpha\beta}} \int_{\Omega} \mathbf{R}_{\alpha\beta} \psi(\mathbf{R}_{\alpha\beta}, \mathbf{r}, \mathbf{p}, t|\mathbf{r}_0, \mathbf{p}_0) d\mathbf{p} d^2\mathbf{r}. \quad (25)$$

The right-hand side in Eq. (25) is nothing but  $\mathbf{M}_1$ . Therefore the asymptotic velocity is

$$\bar{\mathbf{U}} = \lim_{t \rightarrow \infty} \frac{d}{dt} \bar{\Delta \mathbf{R}}(t) = \lim_{t \rightarrow \infty} \frac{d\mathbf{M}_1}{dt} = - \lim_{t \rightarrow \infty} \int_{\Omega} \int_{\partial C_r + \partial C_t} \llbracket \mathbf{J}_1 \rrbracket \cdot \mathbf{n} d\ell d\mathbf{p}, \quad (26)$$

where the last equation results from Eq. (24). Using Eq. (29a) along with boundary conditions (18b) and (19b) we easily show that  $\llbracket \mathbf{J}_1 \rrbracket = -\mathbf{J}_0 \llbracket \mathbf{r} \rrbracket$ , and therefore

$$\bar{\mathbf{U}} = \int_{\Omega} \int_{\partial C_r + \partial C_t} \llbracket \mathbf{r} \rrbracket \mathbf{J}_0^{\infty} \cdot \mathbf{n} d\ell d\mathbf{p}. \quad (27)$$

Evaluating  $\bar{\mathbf{U}}$  using Eq. (27) thus requires solving for the steady-state zeroth-order local moment  $\psi_0^{\infty}(\mathbf{r}, \mathbf{p})$ , which satisfies the steady Fokker-Planck equation

$$\nabla_r \cdot \mathbf{J}_0^{\infty} + \nabla_p \cdot \mathbf{j}_0^{\infty} = 0, \quad (28)$$

with fluxes

$$\mathbf{J}_0^{\infty} = [\text{Pe}_s \mathbf{p} + \mathbf{u}(\mathbf{r})] \psi_0^{\infty} - \kappa^2 \nabla_r \psi_0^{\infty}, \quad (29a)$$

$$\mathbf{j}_0^{\infty} = \frac{1}{2} [\boldsymbol{\Omega}(\mathbf{r}) \times \mathbf{p}] \psi_0^{\infty} - \nabla_p \psi_0^{\infty}. \quad (29b)$$

Asymptotic convergence of  $\psi_0$  towards  $\psi_0^{\infty}$  can be shown to be exponential with respect to time [1]. Equations (28) and (29a)–(29b) can be solved numerically over a unit cell using a finite-volume method, subject to boundary conditions  $\llbracket \psi_0^{\infty} \rrbracket = 0$  and  $\llbracket \nabla_r \psi_0^{\infty} \rrbracket = \mathbf{0}$  on  $\partial C_r, \partial C_t$ ,  $\mathbf{n}_w \cdot \mathbf{J}_0^{\infty} = 0$  on  $\partial C_w$ , and to the normalization condition:

$$\int_{S_t} \int_{\Omega} \psi_0^{\infty} d\mathbf{p} d^2 \mathbf{r} = 1. \quad (30)$$

(2) *Mean dispersivity*: To determine the dispersivity tensor  $\bar{\mathbf{D}}$ , we first calculate the mean-square displacement of a swimmer as

$$\overline{(\Delta \mathbf{R}(t) - \bar{\Delta \mathbf{R}}(t))^2} = \sum_{\alpha, \beta = -\infty}^{\infty} \int_{S_{\alpha\beta}} \int_{\Omega} (\mathbf{R}_{\alpha\beta} - \bar{\Delta \mathbf{R}}(t))^2 \psi(\mathbf{R}_{\alpha\beta}, \mathbf{r}, \mathbf{p}, t | \mathbf{r}_0, \mathbf{p}_0) d\mathbf{p} d^2 \mathbf{r}. \quad (31)$$

Expanding the right-hand side and using the definition of the global moments yields

$$\overline{(\Delta \mathbf{R}(t) - \bar{\Delta \mathbf{R}}(t))^2} = \mathbf{M}_2(t) + \bar{\Delta \mathbf{R}}^2(t) M_0 - \mathbf{M}_1(t) \bar{\Delta \mathbf{R}}(t) - \bar{\Delta \mathbf{R}}(t) \mathbf{M}_1(t) = \mathbf{M}_2(t) - \mathbf{M}_1(t) \mathbf{M}_1(t). \quad (32)$$

We can therefore write the asymptotic dispersivity tensor as

$$\bar{\mathbf{D}} = \lim_{t \rightarrow \infty} \frac{1}{2} \frac{d}{dt} \overline{(\Delta \mathbf{R}(t) - \bar{\Delta \mathbf{R}}(t))^2} = \lim_{t \rightarrow \infty} \frac{1}{2} \frac{d}{dt} (\mathbf{M}_2 - \mathbf{M}_1 \mathbf{M}_1). \quad (33)$$

To make further progress, we first note that integrating Eq. (26) with respect to time gives

$$\mathbf{M}_1(t) = \bar{\mathbf{U}} t + \bar{\mathbf{B}} + \mathcal{O}(e^{-t}), \quad (34)$$

where  $\bar{\mathbf{B}}$  is an unknown constant vector. Recall the definition of  $\mathbf{M}_1(t)$ :

$$\mathbf{M}_1(t) = \int_{S_t} \int_{\Omega} \psi_1(\mathbf{r}, \mathbf{p}, t) d\mathbf{p} d^2 \mathbf{r}. \quad (35)$$

Comparison of Eqs. (34) and (35) suggests seeking the asymptotic solution for  $\psi_1$  in the form

$$\psi_1(\mathbf{r}, \mathbf{p}, t) = \psi_0^{\infty}(\mathbf{r}, \mathbf{p}) [\bar{\mathbf{U}} t + \mathbf{B}(\mathbf{r}, \mathbf{p})] + \mathcal{O}(e^{-t}), \quad (36)$$

where  $\mathbf{B}(\mathbf{r}, \mathbf{p})$  is a vector field to be determined that must satisfy the condition

$$\bar{\mathbf{B}} = \int_{S_t} \int_{\Omega} \psi_0^{\infty} \mathbf{B}(\mathbf{r}, \mathbf{p}) d\mathbf{p} d^2 \mathbf{r}. \quad (37)$$

Using Eq. (35), Eq. (33) thus becomes

$$\overline{\mathbf{D}} = \lim_{t \rightarrow \infty} \frac{1}{2} \frac{d\mathbf{M}_2}{dt} - \overline{\mathbf{U}} \overline{\mathbf{U}} t - \frac{1}{2} (\overline{\mathbf{U}} \overline{\mathbf{B}} + \overline{\mathbf{B}} \overline{\mathbf{U}}). \quad (38)$$

The first term on the right-hand side is estimated using Eq. (24) as

$$\lim_{t \rightarrow \infty} \frac{d\mathbf{M}_2}{dt} = - \lim_{t \rightarrow \infty} \int_{\Omega} \int_{\partial C_r + \partial C_t} [\mathbf{J}_2] \cdot \mathbf{n} d\ell d\mathbf{p}. \quad (39)$$

The jump in  $\mathbf{J}_2$  can be obtained from Eq. (29a). After using boundary conditions (18c)–(19c) along with Eq. (36), it can be expressed as

$$\lim_{t \rightarrow \infty} [\mathbf{J}_2] = -\mathbf{J}_0^\infty (\overline{\mathbf{U}}[\mathbf{r}]t + [\mathbf{r}]\overline{\mathbf{U}}t - [\mathbf{B}\mathbf{B}]) - \kappa^2 \psi_0^\infty [\nabla_r (\mathbf{B}\mathbf{B})]. \quad (40)$$

Inserting this equation into Eqs. (39) and (38) provides the dispersivity in terms of the  $\mathbf{B}$  field as

$$\overline{\mathbf{D}} = \frac{1}{2} \int_{\Omega} \int_{\partial C_r + \partial C_t} [\kappa^2 \psi_0^\infty [\nabla_r (\mathbf{B}\mathbf{B})] - \mathbf{J}_0^\infty [\mathbf{B}\mathbf{B}]] \cdot \mathbf{n} d\ell d\mathbf{p} - \frac{1}{2} (\overline{\mathbf{U}} \overline{\mathbf{B}} + \overline{\mathbf{B}} \overline{\mathbf{U}}). \quad (41)$$

We obtain an equation for  $\mathbf{B}$  by plugging Eq. (36) into the governing equation for  $\psi_1$ . All calculations done, we find

$$-\nabla_r \cdot [\mathbf{J}_0^\infty \mathbf{B} - \kappa^2 \psi_0 \nabla_r \mathbf{B}] - \nabla_p \cdot [\mathbf{j}_0^\infty \mathbf{B} - \psi_0 \nabla_p \mathbf{B}] = \psi_0^\infty \overline{\mathbf{U}}. \quad (42)$$

This equation is also solved numerically using finite volumes, with boundary conditions  $[\mathbf{B}] = -[\mathbf{r}]$  and  $[\nabla_r \mathbf{B}] = \mathbf{0}$  on  $\partial C_r$ ,  $\partial C_t$ , and  $\mathbf{n}_w \cdot \nabla_r \mathbf{B} = \mathbf{0}$  on  $\partial C_w$ . The boundary value problem of Eq. (42) is undetermined as specified. We make it solvable by prescribing the additional condition:

$$\int_{S_t} \int_{\Omega} \mathbf{B}(\mathbf{r}, \mathbf{p}) d\mathbf{p} d^2 \mathbf{r} = \mathbf{k}, \quad (43)$$

where  $\mathbf{k}$  is an arbitrary constant vector that we can set to  $\mathbf{0}$  without loss of generality. Indeed, the choice of  $\mathbf{k}$  does not affect the result for the dispersivity, as  $\overline{\mathbf{D}}$  only depends on the spatial and orientational gradients of  $\mathbf{B}$ .

#### D. Eulerian interpretation of $\overline{\mathbf{U}}$ and $\overline{\mathbf{D}}$

As discussed in the main text, we posit that the long-time transport can be described by an advection-diffusion equation on the Darcy scale. Specifically, we introduce a discrete conditional probability density

$$\Psi(\mathbf{R}_{\alpha\beta}, t | \mathbf{r}_0, \mathbf{p}_0) = \frac{1}{S_t} \int_{\Omega} \int_{S_{\alpha\beta}} \psi(\mathbf{R}_{\alpha\beta}, \mathbf{r}, \mathbf{p}, t | \mathbf{r}_0, \mathbf{p}_0) d^2 \mathbf{r} d\mathbf{p}, \quad (44)$$

which represents the probability for a particle to be located in the cell labeled by the integers  $(\alpha, \beta)$  at time  $t$ , and whose value is assigned to the centroid of the unit cell. On large length scales, we can assimilate  $\mathbf{R}_{\alpha\beta}$  to a continuous variable  $\mathbf{X}$  and define a corresponding macro-scale gradient operator  $\nabla_X$ . The Darcy-scale probability density  $\Psi(\mathbf{X}, t)$ , which is the continuous counterpart of  $\Psi(\mathbf{R}_{\alpha\beta}, t | \mathbf{r}_0, \mathbf{p}_0)$ , is then expected to formally satisfy the 2D obstacle-free advection-diffusion equation

$$\partial_t \Psi + \nabla_X \cdot (\overline{\mathbf{U}} \Psi - \overline{\mathbf{D}} \cdot \nabla_X \Psi) = \delta(\mathbf{X} - \mathbf{X}_0) \delta(t). \quad (45)$$

While a rigorous derivation of Eq. (45) is non-trivial, it is straightforward to verify that its solution has the same global moments as  $\psi$ . In order to show this, we first use Eqs. (8) and (21) to find a relation between the global moments and the discontinuous conditional probability density  $\Psi$ :

$$\mathbf{M}_k(t | \mathbf{r}_0, \mathbf{p}_0) = S_t \sum_{\alpha, \beta = -\infty}^{\infty} \underbrace{\mathbf{R}_{\alpha\beta} \cdots \mathbf{R}_{\alpha\beta}}_{k \text{ times}} \Psi(\mathbf{R}_{\alpha\beta}, t | \mathbf{r}_0, \mathbf{p}_0). \quad (46)$$

The long-time continuous version of Eq. (46) becomes:

$$\mathbf{M}_k(t) = \int_{S_\infty} \underbrace{\mathbf{X} \cdots \mathbf{X}}_{k \text{ times}} \Psi(\mathbf{X}, t) d^2 \mathbf{X}, \quad (47)$$

where the infinite double sum operator has been replaced by an integral over the entire domain. Notice that we have assumed that at long times the dependence of the global moments on the initial conditions disappears. We set  $k = 1$  in Eq. (47) and take the first temporal derivative. In conjunction with Eq. (45), this yields:

$$\lim_{t \rightarrow \infty} \frac{d\mathbf{M}_1}{dt} = - \int_{S_\infty} \mathbf{X} \nabla_{\mathbf{X}} \cdot (\bar{\mathbf{U}}\Psi - \bar{\mathbf{D}} \cdot \nabla_{\mathbf{X}}\Psi) d^2\mathbf{X}. \quad (48)$$

Applying integration by parts and boundary conditions at infinity then gives

$$\lim_{t \rightarrow \infty} \frac{d\mathbf{M}_1}{dt} = \bar{\mathbf{U}}, \quad (49)$$

which is consistent with Eq. (26). Similarly, taking the temporal derivative of  $\mathbf{M}_2(t)$  in Eq. (47) gives

$$\lim_{t \rightarrow \infty} \frac{d\mathbf{M}_2}{dt} = - \int_{S_\infty} \mathbf{X} \mathbf{X} \nabla_{\mathbf{X}} \cdot (\bar{\mathbf{U}}\Psi - \bar{\mathbf{D}} \cdot \nabla_{\mathbf{X}}\Psi) d^2\mathbf{X} = \bar{\mathbf{U}}\mathbf{M}_1 + \mathbf{M}_1\bar{\mathbf{U}} + 2\bar{\mathbf{D}}, \quad (50)$$

which again agrees with Eq. (33).

For an arbitrary incoming flow, the dispersion tensor is non-diagonal but can be expressed as  $\bar{\mathbf{D}} = D_1\mathbf{e}_1\mathbf{e}_1 + D_2\mathbf{e}_2\mathbf{e}_2$  where  $(D_1, D_2)$  are its eigenvalues with corresponding eigenvectors  $(\mathbf{e}_1, \mathbf{e}_2)$ . With these notations, the solution of Eq. (45) for the spreading of a concentrated point source can be expressed as

$$\Psi(\mathbf{X}, t) = \frac{1}{4\pi t \sqrt{D_1 D_2}} \exp \left[ -\frac{(X_1 - U_1 t)^2}{4D_1 t} - \frac{(X_2 - U_2 t)^2}{4D_2 t} \right], \quad (51)$$

where  $(X_1, X_2)$  and  $(U_1, U_2)$  are the components of  $\mathbf{X}$  and  $\bar{\mathbf{U}}$  in the basis of the eigenvectors. Eq. (51) simply states that the particle cloud will spread as a translating anisotropic Gaussian, and a comparison of this solution with results from Brownian dynamics simulations indeed shows excellent agreement at long times in Fig. 2 of the main text.

At pre-asymptotic times, the distributions obtained from simulations are marked by tailed distributions as opposed to the symmetric Gaussian predicted by Eq. (51). In order to characterize these tails and the convergence to the diffusive regime, we study the evolution of the skewness of particle distributions from Brownian dynamics simulations in Fig. 2. A recent experimental study using *E. Coli* reported positively skewed particle distributions [2]. In our simulations, we observe that in strong flows the distributions are always negatively skewed in the direction of the flow as more particles tend to accumulate downstream. However, for strong swimming or weak flow the distributions are found to be positively skewed. As seen in Fig. 2, the skewness eventually approaches zero as the diffusive regime is reached.

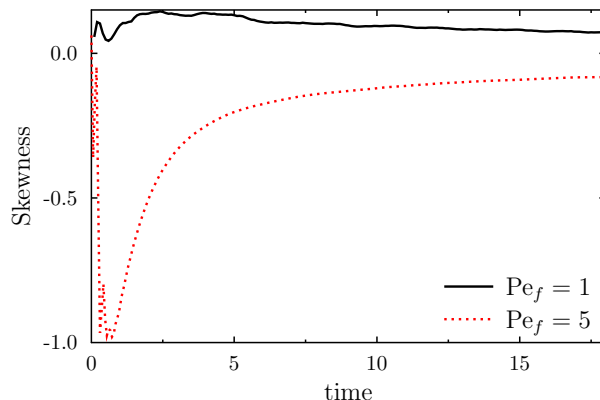

FIG. 2: Evolution of the skewness of particle distributions over time as calculated from Brownian dynamics simulations. Parameter values:  $\text{Pe}_s = 1$ ,  $\kappa^2 = 0.1$ ,  $\Theta_f = 0$ ,  $\epsilon_p = 0.804$ .

## II. Flow calculation: boundary integral method

We use the boundary integral method [3] to calculate the fluid velocity. Owing to the periodicity of the lattice, we can make use of the doubly periodic Green's function for two-dimensional Stokes flow, which is computed using standard

Ewald summation techniques. The fluid velocity  $\mathbf{u}$  at any point inside the unit cell of the lattice is decomposed into the free-stream component  $\mathbf{u}^\infty$  and a disturbance velocity  $\mathbf{u}^D$  generated due to the presence of the obstacles. In the present problem we take  $\mathbf{u}^\infty$  to be a uniform streaming flow. On the surface  $\partial C_w$  of the obstacles, the no-slip condition  $\mathbf{u} = 0$  is satisfied, or alternately,  $\mathbf{u}^D = -\mathbf{u}^\infty$ . We use a single-layer representation for the velocity to obtain:

$$\mathbf{u}(\mathbf{x}_0) = \mathbf{u}^\infty(\mathbf{x}_0) - \frac{1}{4\pi\mu} \sum_{q=0}^{N_p} \int_{C_q} \mathbf{G}(\mathbf{x}, \mathbf{x}_0) \cdot \mathbf{f}(\mathbf{x}) d\ell(\mathbf{x}), \quad (52)$$

where  $N_p$  is the total number of obstacles within the unit cell,  $C_q$  is the contour of the  $q^{th}$  obstacle,  $\mathbf{G}(\mathbf{x}, \mathbf{x}_0)$  is the computed Green's function, and  $\mathbf{f}(\mathbf{x})$  is the local traction. On enforcing the no-slip boundary condition one is able to solve for unknown tractions by inverting a dense linear system. Once the tractions are obtained, the fluid velocity can be calculated at any point using Eq. (52). For all the cases presented in the paper we have used linear elements to discretize the contour of the obstacles and Gauss-Legendre quadrature for evaluating the integrals. Sangani and Acrivos [4] studied the flow past a periodic array of circular cylinders using the streamfunction-vorticity formulation and provided the results for drag on a cylinder as a function of obstacle volume fraction: our numerical method was validated against their results and excellent agreement was found.

In order to facilitate fast computation, the velocity was pre-tabulated on a Cartesian mesh and bilinear interpolation was used subsequently. We used second-order-accurate finite-difference approximations to compute and tabulate gradients on the mesh. Our interpolation results were validated against the boundary integral method and the error was always within one percent.

### III. Conformal mapping for non-circular obstacles

In order to explore the possibility of guiding, trapping or controlling the spread of active particles, we consider a number of non-circular pillar geometries in Figs. 1 and 4 of the main text, which were obtained using conformal mappings. Specifically, we make use of following Riemann map of the unit disc:

$$z(\sigma) = \mathcal{W}\sigma + \frac{\mathcal{Y}}{\sigma} + \frac{\mathcal{Z}}{\sqrt{2}\sigma^2}, \quad (53)$$

where  $\sigma = e^{i\chi}$  with polar angle  $\chi \in [0, 2\pi)$ .  $\{\mathcal{W}, \mathcal{Y}, \mathcal{Z}\}$  are three parameters that are varied to change the obstacle shape. An identical conformal map was previously used to study amoeboid swimming [5]. Avoiding self-intersection of the boundary provides the following constraint on the shape parameters [5]:

$$\mathcal{W} \geq \mathcal{Y} \pm \sqrt{2}\mathcal{Z}, \quad \mathcal{W}\mathcal{Y} \geq 2\mathcal{Z}^2 - \mathcal{W}^2. \quad (54)$$

For a given lattice porosity we also need to constrain the area of these shapes. It can be shown [5] that the area of any of these shapes is given by:

$$A = \pi (\mathcal{W}^2 - \mathcal{Y}^2 - \mathcal{Z}^2). \quad (55)$$

Following our non-dimensionalization, we chose the area  $A$  to be identical to a circle with unit radius. Given the value of  $A$ , we need only vary parameters  $\{\mathcal{Y}, \mathcal{Z}\}$ , which control shape aspect ratio and fore-aft asymmetry, respectively.

### IV. Brownian dynamics algorithm

In two dimensions, the Langevin equations for the dynamics of an active Brownian swimmer located at position  $\mathbf{r}$  with orientation  $\mathbf{p} = (\cos \theta, \sin \theta)$  can be written as

$$\dot{\mathbf{r}} = v_0 \mathbf{p} + \mathbf{u}(\mathbf{r}) + \boldsymbol{\eta}_t, \quad (56)$$

$$\dot{\theta} = \mathbf{p}^\perp \cdot \nabla \mathbf{u}^T \cdot \mathbf{p} + \eta_r, \quad (57)$$

where  $\mathbf{p}^\perp \equiv (-\sin \theta, \cos \theta)$ . The two noise terms  $\boldsymbol{\eta}_t$  and  $\eta_r$  capture thermal fluctuations and must obey the fluctuation-dissipation theorem:

$$\langle \boldsymbol{\eta}_t(t) \rangle = \mathbf{0}, \quad \langle \eta_r(t) \rangle = 0, \quad (58)$$

$$\langle \boldsymbol{\eta}_t(t) \boldsymbol{\eta}_t(t') \rangle = \sqrt{2d_t} \mathbf{I} \delta(t - t'), \quad (59)$$

$$\langle \eta_r(t) \eta_r(t') \rangle = \sqrt{2d_r} \delta(t - t'), \quad (60)$$

where  $d_t$  and  $d_r$  are the translational and rotational diffusivities. Using the appropriate length and time scales of the model it is possible to obtain the dimensionless Langevin equations. During time step  $\Delta t$  in a simulation, we calculate the changes in position and orientation as follows:

$$\Delta \mathbf{x} = [\text{Pe}_s \mathbf{p} + \text{Pe}_f \mathbf{u}] \Delta t + \sqrt{2\kappa^2 \Delta t} \boldsymbol{\zeta}_t, \quad (61)$$

$$\Delta \theta = [\mathbf{p}^\perp \cdot \nabla \mathbf{u}^T \cdot \mathbf{p}] \Delta t + \sqrt{2\Delta t} \zeta_r, \quad (62)$$

where the equations have been made dimensionless, and where  $\boldsymbol{\zeta}_t$  and  $\zeta_r$  are Gaussian random variables with zero mean and unit variance. In most of our simulations we used  $N = 10^5$  particles. The no-flux boundary condition on the surface of the obstacles is enforced using reflecting boundaries. The Brownian simulations were validated against well-known results for passive tracer transport in porous media [6].

### V. Upstream vs downstream swimming

The fraction of time  $\tau^{up}$  spent by the particles moving upstream ( $\Delta \mathbf{x} \cdot \mathbf{e}_x < 0$ ) is shown in Fig. 3. We obtain  $\tau^{up}$  from the macrotransport theory as:

$$\tau^{up} = \int_{S_t} \int_{\Omega} \psi_0^\infty(\mathbf{r}, \mathbf{p} | \mathbf{J}_0^\infty \cdot \mathbf{e}_x < 0) d\mathbf{p} d^2\mathbf{r}. \quad (63)$$

For a purely diffusive process in the absence of any flow, the particles are equally likely to go upstream or downstream and therefore  $\tau^{up} = 0.5$ . For weak swimming, particles get washed out by the flow. As  $\text{Pe}_f$  increases, more particles go downstream due to a strong shear, and they eventually behave as passive tracers for sufficiently high  $\text{Pe}_f$ . For strong swimming, shear-induced rotations promote upstream swimming, which results in an initial increase in  $\tau^{up}$ , as observed in Fig. 3 for  $\text{Pe}_s = 5$  and 10. Our results are in good qualitative agreement with recently reported experimental results for the transport of *E. Coli* under strong flows [2].

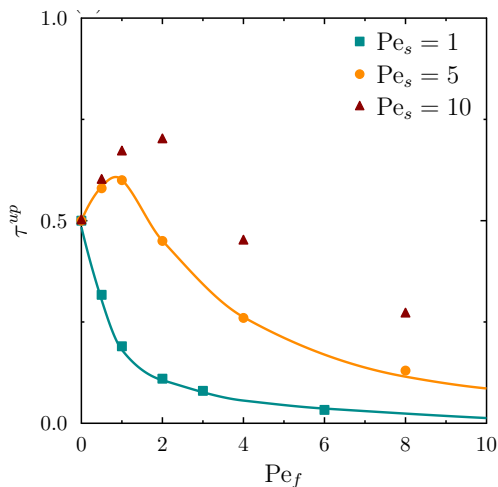

FIG. 3: Fraction of time  $\tau^{up}$  during which particles are oriented upstream, as a function of  $\text{Pe}_f$  for different activity levels. Symbols correspond to Brownian dynamics simulations and the lines are results from the macro-transport theory. Parameter values:  $\kappa^2 = 0.1$ ,  $\Theta_f = 0$ ,  $\epsilon_p = 0.804$ .

- 
- [1] H. Brenner, Phil. Trans. R. Soc. Lond. A **297**, 81 (1980).
  - [2] A. Creppy, E. Clément, C. Douarche, M. V. D'Angelo, and H. Auradou, arXiv preprint arXiv:1802.01879 (2018).
  - [3] C. Pozrikidis, *Boundary Integral and Singularity Methods for Linearized Viscous Flow* (Cambridge University Press, 1992).
  - [4] A. Sangani and A. Acrivos, Intl. J. Multiphase Flow **8**, 193 (1982).
  - [5] J. Avron, O. Gat, and O. Kenneth, Phys. Rev. Lett. **93**, 186001 (2004).
  - [6] D. Edwards, M. Shapira, H. Brenner, and M. Shapira, Trans. Porous Media **6**, 337 (1991).
